# Supplementary material for: Source-free Video Domain Adaptation by Learning from Noisy Labels
Source: arXiv:2311.18572 source file (2025-11-28)
Supplement: Supplementary file 1 [file epic-additional.tex]

\setlength{\tabcolsep}{4pt}
\begin{table*}[htp]
% \scriptsize
\centering
\caption{Performance comparisons with state-of-the-art video domain adaptation methods on EPIC-Kitchens dataset. All models reported are single-stream (appearance) networks. The results for our methods are highlighted in \textcolor{gray}{gray} color.}

\begin{tabular}{cclllllll}
\hline
 \textbf{Method} & \textbf{Source-free?} &\textbf{D2$\rightarrow$D1} & \textbf{D3$\rightarrow$D1} & \textbf{D1$\rightarrow$D2} & \textbf{D3$\rightarrow$D2} & \textbf{D1$\rightarrow$D3} & \textbf{D2$\rightarrow$D3} & \textbf{Mean}   \\ \hline 
Source only & &  35.4 &  34.6 &32.8  & 35.8&34.1  &39.1  & 35.3 \\ 

DANN~\cite{ganin2015unsupervised} & \textcolor{red}{\xmark}& 38.3 & 38.8 & 37.7 & 42.1&36.6 &41.9 &39.2\\

ADDA~\cite{tzeng2017adversarial} &\textcolor{red}{\xmark} & 36.3  & 36.1 & 35.4 & 41.4& 34.9& 40.8&37.4 \\

TA3N~\cite{chen2019temporal} &\textcolor{red}{\xmark} & 40.9& 39.9&34.2 &44.2 &37.4 &42.8 & 39.9 \\

CoMix~\cite{sahoo2021contrast}  &\textcolor{red}{\xmark} & 38.6 &42.3 & 42.9 &49.2 &40.9 &45.2 &43.2 \\ 

 Target Supervised& & 57.0 & 57.0 & 64.0 & 64.0 & 63.7 & 63.7   & 61.5\\ \hline
 
 \rowcolor{Gray}
 Source only & & 40.9 & 38.6 & 39.3 & 41.3 & 37.3 & 42.4 & 39.9 \\ \rowcolor{Gray}
 \method{} & \textcolor{green}{\cmark} &  44.6 \textcolor{ForestGreen}{$\blacktriangle \text{+} 3.7$}& 40.7 \textcolor{ForestGreen}{$\blacktriangle \text{+}2.1$ } &  44.5 \textcolor{ForestGreen}{$\blacktriangle \text{+} 5.2$} &  47.1 \textcolor{ForestGreen}{$\blacktriangle \text{+}5.8$ }&  40.9 \textcolor{ForestGreen}{$\blacktriangle \text{+}3.6$ } & 45.7 \textcolor{ForestGreen}{$\blacktriangle \text{+}3.3$}&  43.9 \textcolor{ForestGreen}{$\blacktriangle \text{+} 4.0$}  \\ \rowcolor{Gray}
 Target Supervised & & 60.5 & 60.5 & 68.4  & 68.4 & 68.8  & 68.8  &  65.9 \\ \hline
\end{tabular}
\label{tab:epic-additional}
% \vspace{-0.6cm}
\end{table*}
